# Supplementary material for: On the Interplay of Regional Mobility, Social Connectedness, and the Spread of COVID-19 in Germany
Source: arXiv:2008.03013 source file (2021-07-02)

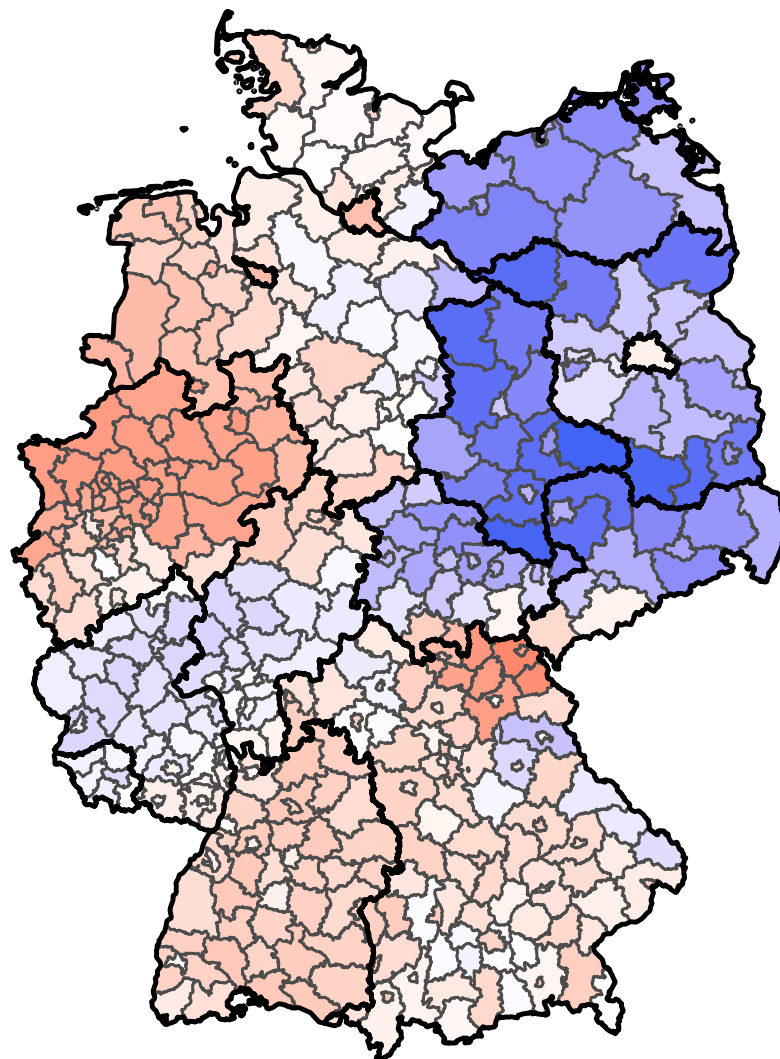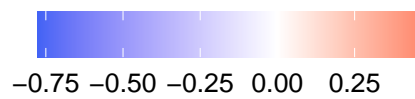

(a) Long Term Effect

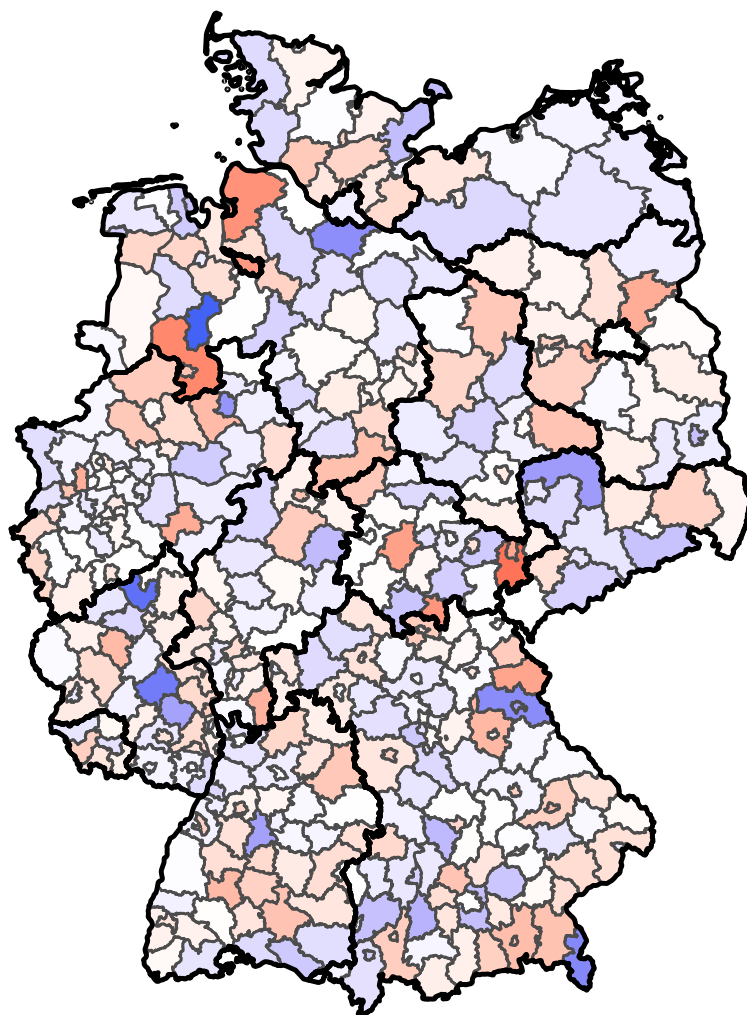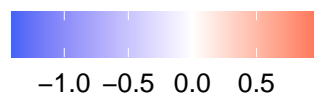

(b) Short Term Effect

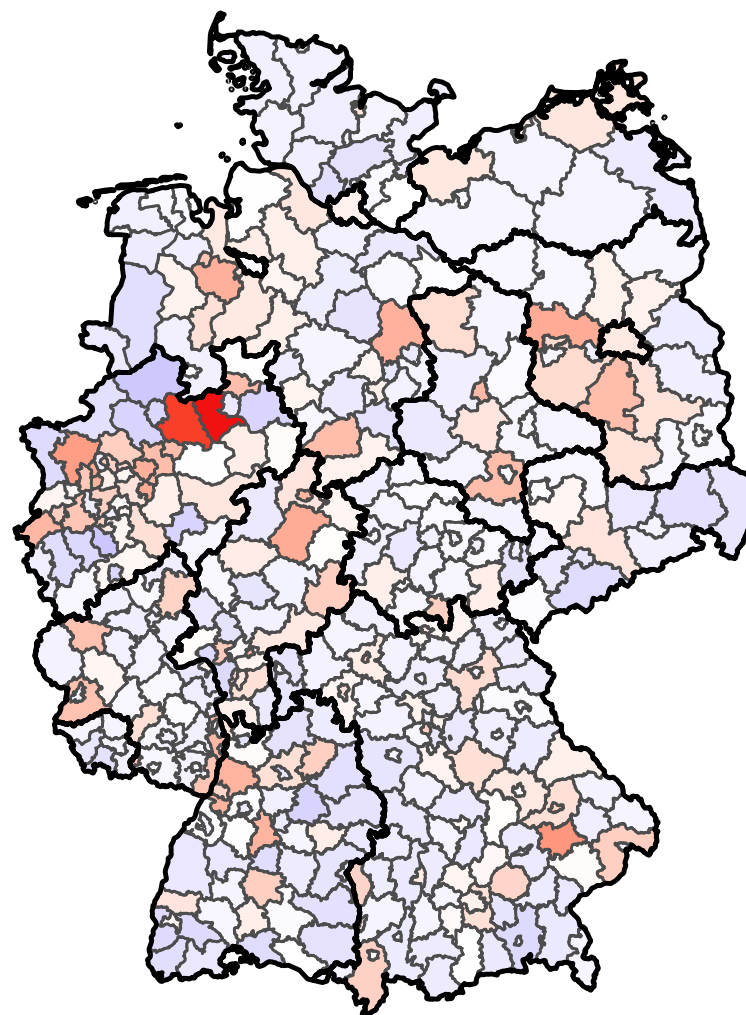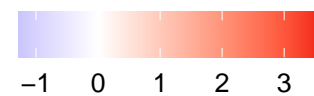

Supplement: Supplementary file 1 [file sm_figure_12_13.pdf]
