# Supplementary material for: On the Interplay of Regional Mobility, Social Connectedness, and the Spread of COVID-19 in Germany
Source: arXiv:2008.03013 source file (2021-07-02)

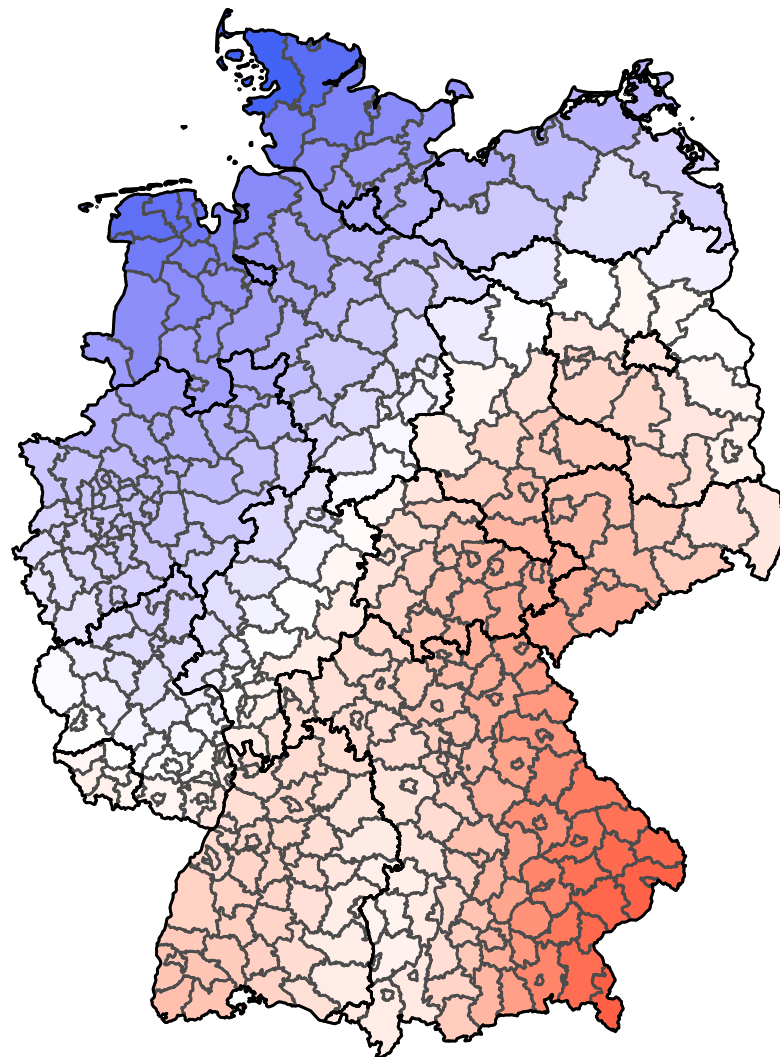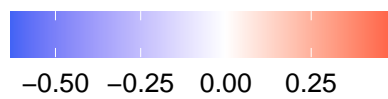

(c) Long Term Random Effect

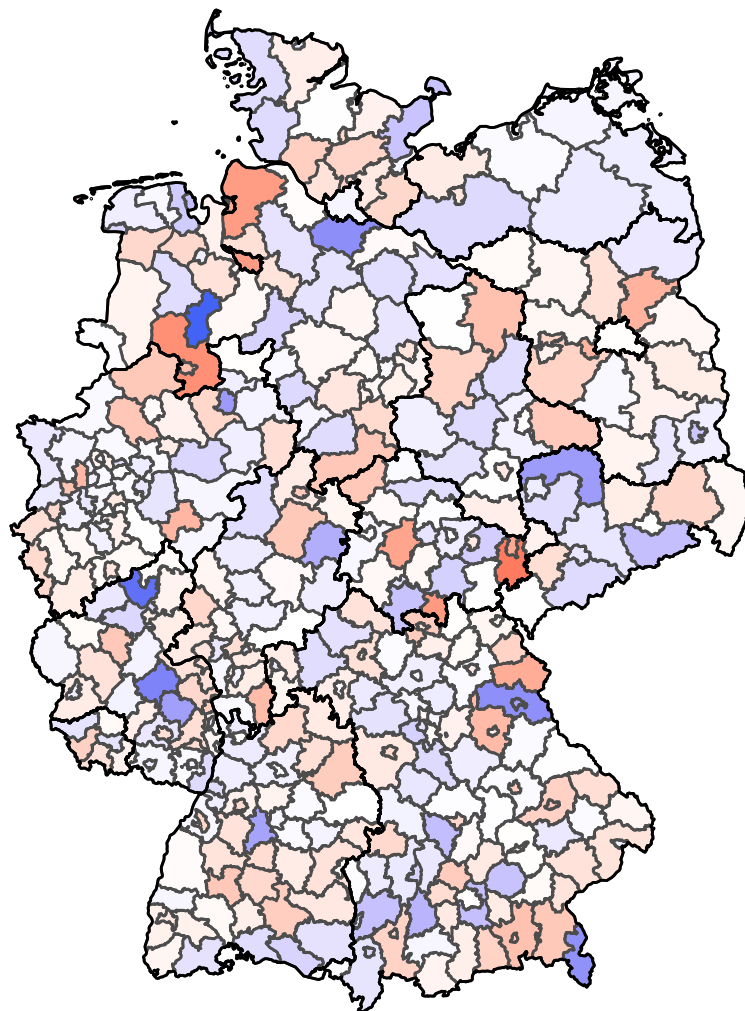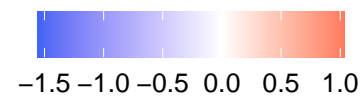

(d) Short Term Random Effect

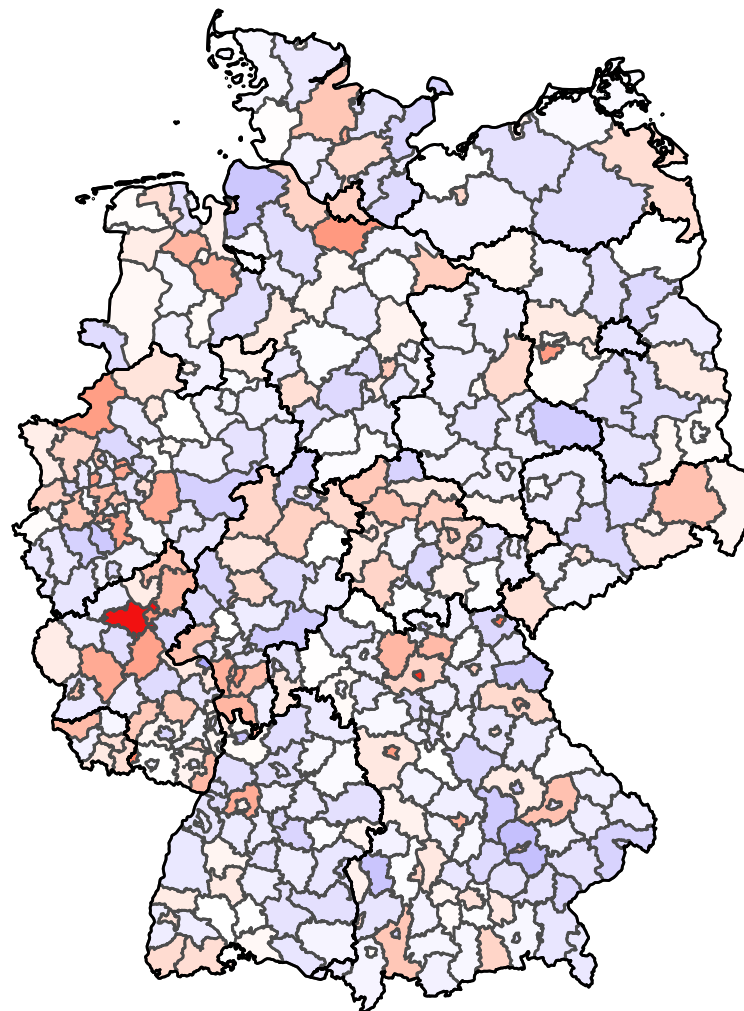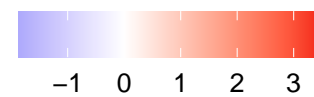

Supplement: Supplementary file 2 [file suppl_furtherresults.pdf]
